# Supplementary material for: Plan-Driven Adaptive Bidding for First-Price Auctions with Budget Constraints under Nonstationarity
Source: arXiv:2505.02796 source file (2026-09-20)
Supplement: Supplementary file 1 [file appendix.tex]

\newpage
\onecolumn
\setcounter{section}{0}

\section{Proof of Theorem \ref{thrm:noninformative}}\label{proof3.1}

We consider an alternate system and the performance of \Cref{alg:1} in the alternate system provides a lower bound on the performance $\Vpi$
of \Cref{alg:1} in the original system.
Therefore, we can bound $\Vpi$ from below by bounding the performance of \Cref{alg:1} in the alternate system.

Specifically, we consider an alternate system where (i) there is no budget constraint -- i.e., the remaining budget can go negative;
however, (ii) whenever the payment exceeds the remaining budget, i.e., $z_t > B_t$, a penalty $b$ (which is an upper bound on
the private values) will occur, making the net reward negative.

In the following, we use a superscript $R$ to denote the dynamics in the alternate system. We let $\BR_t$ denote the value of the remaining budget at the beginning of period $t$ of the alternate system,
and we let $\xR_t$, $\zR_t$, $\gR_t = \rho - \zR_t$, and $\muR_t$, respectively,  denote the bid, consumption, gradient, and dual variable in period $t$ of the alternate system.
Note that since there is no budget constraint in the alternate system, \Cref{alg:1} always proceeds with
$\xR_t \triangleq \text{argmax}_{x \in [a,b]} \big(v_t - (1 + \muR_t) x\big) {G}_t(x)$ and $\muR_{t+1} = (\muR_t - \eta \gR_t)^{+}$ for all periods $t \in [T]$.

Note that the cumulative reward of \Cref{alg:1} is lower in the alternate system than in the original system for every sample path. To see this, consider a critical period $\tau = \min\{t: \zR_t > \BR_t\}$, which is the first time that the remaining budget in the alternate system becomes negative.
Note that the two systems collect the same reward in each period until period $\tau - 1$. Moving forward, the bidder in the original system still collects a nonnegative reward in each remaining period. In contrast, the net reward in each remaining period of the alternate system is always nonpositive because of the penalty $-b$ of winning an auction when the budget is exhausted.

Since the performance of \Cref{alg:1} in the alternate system is a lower bound on the performance $\Vpi$ of \Cref{alg:1} in the original system, we have
\begin{equation*}
\begin{aligned}
\Vpi &\geq \E\left\{\sum_{t \in [T]}(v_t - \xR_t) \mathbf{1}[\xR_t \geq m_t] - \sum_{t \in [T]}b \cdot \mathbf{1}[\xR_t \geq m_t]\mathbf{1}\big[\xR_t > \BR_t\big]\right\} \\
&\geq
\E\left[\sum_{t \in [T]}(v_t - \xR_t) G(\xR_t)\right] - b \cdot \E\left[ \frac{(\sum_{t=1}^T \zR_t - B)^{+}}{a} + 1\right].
\end{aligned}
\end{equation*}
As a result,
\begin{equation}\label{eq:tmp1}
\VOPT - \Vpi \leq \underbrace{\VOPT - \E\left[\sum_{t \in [T]}(v_t - \xR_t) G(\xR_t) \right]}_{(a)}
+ \underbrace{b \cdot \E\left[ \frac{(\sum_{t=1}^T \zR_t - B)^{+}}{a} + 1\right]}_{(b)}.
\end{equation}

In the following, we analyze the alternate system and show that $(a) = O(\sqrt{T\ln T}) + 2\mathcal{W}_T$ (\Cref{appx:subsec:term-a}) and $b = O(\sqrt{T})$ (\Cref{appx:subsec:term-b}), with which we prove the result.
We first provide some auxiliary lemmas in \Cref{appx:subsec:prep-unknown-F} for preparation.

\subsection{Auxiliary Lemmas}\label{appx:subsec:prep-unknown-F}

\begin{lemma}\label{lemma:bdd-mu}
If the initial dual variable $\mu_1 \leq \frac{b}{a} + b$ and the step size $\eta \leq 1$, then the dual variables $\mu_t \leq \frac{b}{a} + b$ are uniformly bounded from above for all $t \geq 1$.
\end{lemma}
\begin{proof}{Proof:}
It suffices to show that if $\muR_t \leq \frac{b}{a} + b$, then $\muR_{t+1} \leq \frac{b}{a} + b$ as well. To see this,
first, if $\muR_t \in  [\frac{b}{a}, \frac{b}{a} + b]$, then $\xR_t \triangleq \text{argmax}_{x \in [a,b]} \big(v_t - (1 + \muR_t) x\big) {G}_t(x) = 0$.
As a result,
$\gR_t = \rho > 0$ and $\muR_{t+1} = (\muR_t - \eta \gR_t)^{+} \leq \muR_t \leq \frac{b}{a} + b$.
Next, suppose that $\muR_t \leq \frac{b}{a}$ and $\eta \leq 1$.
Since $\gR_t = \rho - \xR_t\mathbf{1}[\xR_t \geq m_t] \geq -b$, we have
$\muR_{t+1} = (\muR_t - \eta \gR_t)^{+} \leq \muR_t + b \leq \frac{b}{a} + b$.
\end{proof}

We introduce the well-known Dvoretzky-Kiefer-Wolfowith inequality in Lemma \ref{lemma:DKW_ineq} to bound the error of estimating the distribution $G(\cdot)$ using its empirical distribution.

\begin{lemma}[Dvoretzky-Kiefer-Wolfowith Inequality]\label{lemma:DKW_ineq}
Let $G(x)$ be a one-dimensional cumulative distribution function,
and $G_n(x)$ be an empirical cumulative distribution function from $n$ $i.i.d.$ samples of $G(x)$. Then,
for any $n > 0$ and $\epsilon > 0$,
\begin{equation*}
\p\left[ \sup_{x \in \mathbb{R}} \big|G_n(x) - G(x)\big| \geq \epsilon \right] \leq 2 e^{-2n\epsilon^2}.
\end{equation*}
\end{lemma}

Let $err_G(t) \triangleq \sup_{x \in [a,b]} \big|{G}_{t}(x) - G(x)\big|$ denote the estimation error regarding the distribution $G$ in period $t$.
From Lemma \ref{lemma:DKW_ineq} and the union bound we have, with probability at least $1 - \frac{1}{T}$,
$err_G(t+1) \leq \sqrt{\frac{\ln2 + 2 \ln T}{2t}}$ for all periods $t \in [T]$.
Therefore, we have
\begin{equation}\label{eq:est-err}
\E \sum_{t=1}^T \left[err_G(t) \right] \leq 2 + \sum_{t=1}^{\infty} \sqrt{\frac{\ln2 + 2 \ln T}{2t}} = O\big(\sqrt{T\ln T}\big).
\end{equation}

Finally, for any dual variable $\mu \in \mathbb{R}_{+}$ and private-value distribution $F(\cdot)$, we let
\begin{equation}\label{eq:def-L}
L(\mu, F) \triangleq \E_{v \sim F}\left[\big(v - (1 + \mu) x^*(v,\mu)\big) G\big(x^*(v,\mu)\big) \right]
\end{equation}
denote the Lagrangian-adjusted expected reward under the private-value distribution $F(\cdot)$.
Note that the period-$t$ problem $D_t(\mu)$ in the Lagrangian relaxation (as defined in (\ref{eq:offlineLR2})) can be expressed as
$D_t(\mu) = \mu \rho + L(\mu, F_t)$.
\Cref{lemma:W-dist} shows that the function $L(\mu, F)$ is Lipschitz-continuous with respect to distribution $F$ in terms of the Wasserstein distance.
\begin{lemma}\label{lemma:W-dist}
For any two private-value distributions $F_1$ and $F_2$, we have
\begin{equation*}
\sup_{\mu \geq 0} |L(\mu, F_1) - L(\mu, F_2)| \leq \mathcal{W}(F_1, F_2).
\end{equation*}
\end{lemma}
\begin{proof}{Proof of Lemma \ref{lemma:W-dist}}
The proof is analogous to proof of Lemma 3 in \cite{jiang2020online}, and we omit the detail here.
Note that in our setting, the expected budget consumption in a period $t$ is $x_t G(x_t)$, which is independent of the private value $v_t$.
\end{proof}

\subsection{Upper Bound on Term $(a)$}\label{appx:subsec:term-a}

Let
$f^{*}(v, \mu) \triangleq \max_{x \in [a,b]} (v - (1+\mu)x) G(x)$ denote the optimization problem solved in each period of $\VLR(\mu)$,
and recall that $x^*(v, \mu) = \text{argmax}_{x \in [a,b]} (v_t - (1 - \mu) x) G(x)$ denotes the optimal solution.
We can bound the single-period expected reward from below, as follows:
\begin{equation*}\label{eq:one-period-bdd}
\begin{aligned}
&(v_t - \xR_t) G(\xR_t) \\
=& (v_t - (1 + \muR_t)\xR_t) {G}_t(\xR_t)  + \muR_t \xR_t G(\xR_t) + (v_t - (1+\muR_t)\xR_t)\Big( G(\xR_t)  - {G}_t(\xR_t)\Big)\\
\geq& (v_t - (1 + \muR_t) x^*(v_t, \muR_t)) {G}_t(x^*(v_t, \muR_t))  + \muR_t \xR_t G(\xR_t) + (v_t - (1+\muR_t)\xR_t)\Big( G(\xR_t)  - {G}_t(\xR_t)\Big)\\
=& (v_t - (1 + \muR_t) x^*(v_t, \muR_t)) {G}(x^*(v_t, \muR_t)) + (v_t - (1+\muR_t)\xR_t)\Big( G(\xR_t)  - {G}_t(\xR_t)\Big) \\
&+ \muR_t \xR_t G(\xR_t) + (v_t - (1 + \muR_t)x^*(v_t, \muR_t)) \Big({G}_t(x^*(v_t, \muR_t))  - G(x^*(v_t, \muR_t))\Big) \\
\geq& f^*(v_t, \muR_t) + \muR_t \xR_t G(\xR_t) - 2b \cdot err_G(t)
\end{aligned}
\end{equation*}
where the first inequality follows from the definiton $\xR_t = \text{argmax}_{x \in [a,b]} \big(v_t - (1 + \muR_t) x\big) {G}_t(x)$
and the second inequality follows from the definition of $err_G(t) = \sup_{x \in [a,b]} \big|{G}_{t}(x) - G(x)\big|$.

As a result,
\begin{equation}\label{eq:tmp7}
\begin{aligned}
(a) \leq& \VOPT - \E\left[\sum_{t=1}^T f^*(v_t, \muR_t) + \muR_t \rho \right]
+ \E\left[\sum_{t=1}^T \muR_t (\rho - \xR_t G(\xR_t))\right] + 2b \cdot \E\left[\sum_{t=1}^{T} err_G(t)\right] \\
\leq& \underbrace{\VOPT - \E\left[\sum_{t=1}^T f^*(v_t, \muR_t) + \muR_t \rho \right]}_{(c)}
+ \underbrace{\E\left[\sum_{t=1}^T \muR (\rho - \xR_t \mathbf{1}[\xR_t \geq m_t])\right]}_{(d)} + O(\sqrt{T \ln T})
\end{aligned}
\end{equation}
where the second inequality follows from (\ref{eq:est-err}). We now bound the terms $(c)$ and $(d)$ from above.

\paragraph{Upper Bound on Term $(c)$.}
Since $\muR_t$ and $v_t$ are independent, we have
\begin{equation}\label{eq:tmp2}
E[f^*(v_t, \muR_t)] = E_{\muR_t}\big[ L(\muR_t, F_t) \big] \geq
E_{\muR_t}\big[ L(\muR_t, \bar{F}_T) \big] - \mathcal{W}(F_t, \bar{F}_T)
\end{equation}
where the inequality follows from Lemma \ref{lemma:W-dist}.
Let $\bar{\mu} = \frac{1}{T}\sum_{t=1}^{T} \muR_t$ be the mean value of the dual variables $\muR_t$. We have
\begin{equation}\label{eq:tmp3}
\begin{aligned}
\E\left[\sum_{t=1}^T f^*(v_t, \muR_t) + \muR_t \rho \right] &\geq
\E\left[\sum_{t=1}^T \left(L(\muR_t, \bar{F}_T) + \muR_t \rho \right) \right] - \mathcal{W}_T(\mathcal{F}) \\
&\geq T\E\big[\left(L(\bar{\mu}, \bar{F}_T) + \bar{\mu} \rho \right) \big] - \mathcal{W}_T(\mathcal{F})
\end{aligned}
\end{equation}
where the first inequality follows from (\ref{eq:tmp2}), and the second inequality follows from the fact that
$L(\mu, F)$ is convex in $\mu$ and the Jensen's inequality.

On the other hand, since $\VOPT \leq \VLR(\mu)$ for any $\mu \geq 0$ (Lemma \ref{lemma:weak-duality})
and $\VLR(\mu) = \sum_{t=1}^T  D_t(\mu) = \sum_{t=1}^T \Big\{L(\mu, F_t) + \mu \rho \Big\}$,
we have
\begin{equation}\label{eq:tmp4}
\begin{aligned}
    \VOPT & \leq \E[\VLR(\bar{\mu})] = \sum_{t=1}^T \E\Big[L(\bar{\mu}, F_t) + \rho \bar{\mu} \Big] \\
    & \leq \sum_{t=1}^T \left\{ \E\Big[L(\bar{\mu}, \bar{F}_T)  + \rho \bar{\mu} \Big] + \mathcal{W}(F_t, \bar{F}_T) \right\} \\
    & = T\E\left[\left(L(\bar{\mu}, \bar{F}_T) + \bar{\mu} \rho \right) \right] + \mathcal{W}_T(\mathcal{F})
\end{aligned}
\end{equation}
where the second inequality follows from Lemma \ref{lemma:W-dist}.
From (\ref{eq:tmp3}) and (\ref{eq:tmp4}), we have
\begin{equation}\label{eq:tmp5}
(c) \leq 2 \mathcal{W}_T(\mathcal{F}).
\end{equation}

\paragraph{Upper Bound on Term $(d)$.}
Since $\muR_{t+1} = (\muR_t - \eta \gR_t)^{+}$, $\gR_t = \rho - \xR_t \mathbf{1}[\xR_t \geq m_t]$,
and $|\gR_t| \leq C_1 \triangleq \max\{\rho, b - \rho\}$,
we have
\begin{equation*}
(\muR_{t+1})^2 \leq (\muR_{t})^2 + C_1^2\eta^2  - 2 \eta \muR_t (\rho - \xR_t \mathbf{1}[\xR_t \geq m_t]).
\end{equation*}
By telescoping over $t \in [T]$, we have
\begin{equation*}
\begin{aligned}
\sum_{t=1}^T \muR (\rho - \xR_t \mathbf{1}[\xR_t \geq m_t]) \leq \frac{C_1^2}{2} \cdot \eta T + \frac{\mu_1^2}{2\eta}.
\end{aligned}
\end{equation*}
Therefore, by taking $\eta = \frac{1}{\sqrt{T}}$,
\begin{equation}\label{eq:tmp6}
(d) \leq \frac{C_1^2}{2} \cdot \eta T + \frac{\mu_1^2}{2\eta} = O(\sqrt{T}).
\end{equation}
From (\ref{eq:tmp7}), (\ref{eq:tmp5}), and (\ref{eq:tmp6}), we have
\begin{equation*}
(a) = O(\sqrt{T \ln T}) + 2 \mathcal{W}_T(\mathcal{F}).
\end{equation*}

\subsection{Upper Bound on Term $(b)$}\label{appx:subsec:term-b}
Since $\muR_{t+1} = (\muR_t - \eta g_t)^{+} \geq \muR_t - \eta g_t = \muR_t - \eta (\rho - \zR_t)$
and $\rho = \frac{B}{T}$, by telescoping over $t$, we have
\begin{equation*}
\sum_{t=1}^T \zR_t - B = \sum_{t=1}^T \left(\zR_t - \rho \right)
\leq \frac{\muR_{T+1} - \mu_1}{\eta} \leq \frac{b/a+b}{\eta}
\end{equation*}
where the last equality follows from Lemma \ref{lemma:bdd-mu}.
As a result, if we take the step size $\eta = \frac{1}{\sqrt{T}}$,
\begin{equation*}
(b) = O\left(\frac{1}{\eta}\right) = O(\sqrt{T}).
\end{equation*}

\section{Proof of Proposition \ref{prop:lbd-W}}
We separate the proof into two parts:(i)the regret is lower bounded by $\Omega(W_T)$, and (ii)the regret is lower bounded by $\Omega(\sqrt{T})$. By combining the two parts, we prove our results. It is folklore in the literature that no online policy can break the lower bound $\Omega(\sqrt{T})$. Therefore, it only remains to prove the lower bound of $\Omega(W_T)$.

To simplify the proof, here we assume $a=0, b=1$, and denote the reward and consumption at each time period $t$ as $f_t(x_t) = (v_t - x_t) \cdot \mathbf{1}[x_t \geq m_t]$ and $g_t(x_t) = x_t \mathbf{1}[x_t \geq m_t] = z_t$.

We consider the scenario when $m_t = \frac{1}{2}$ for each $t$. That is, when $x_t < \frac{1}{2}$, we have $\mathbf{1}[x_t \geq m_t] = 0$ and $f_t(x_t) = g_t(x_t) = 0$; when $x_t \geq \frac{1}{2}$, we have $\mathbf{1}[x_t \geq m_t] = 1$ and $f_t(x_t) = v_t - x_t, g_t(x_t) = x_t$. For $x_t \geq \frac{1}{2}$, the optimal policy is always to set $x_t = \frac{1}{2}$ to maximize the reward and minimize the consumption.

Set the budget constraint $B = T/4$. Now we consider the following two scenario. The first one, given in (\ref{s1}), is that $v_t = \frac{3}{4}$ for the first half of time horizon $t=1, \cdots, \frac{T}{2}$ and $v_t = \frac{3}{4} + W_T/T$ for the second half of time horizon $t=\frac{T}{2}+1, \cdots, T$. The second scenario, given in (\ref{s2}), is that $v_t = \frac{3}{4}$ for $t=1, \cdots, \frac{T}{2}$ and $v_t = \frac{3}{4} - W_T/T$ for $t=\frac{T}{2}+1, \cdots, T$.

\begin{equation} \label{s1}
    \begin{aligned}
       max \ \ & (\frac{3}{4} - x_1)\mathbf{1}[x_1 \geq \frac{1}{2}] + \cdots + (\frac{3}{4} - x_{\frac{T}{2}})\mathbf{1}[x_{\frac{T}{2}} \geq \frac{1}{2}] \\
       & + (\frac{3}{4}+\frac{W_T}{T} - x_{\frac{T}{2}+1})\mathbf{1}[x_{\frac{T}{2}+1} \geq \frac{1}{2}] + \cdots + (\frac{3}{4}+\frac{W_T}{T} - x_T)\mathbf{1}[x_T \geq \frac{1}{2}] \\
       s.t. \ \ & \sum_{t=1}^T g_t(x_t)  \leq \frac{T}{4} , \ 0 \leq x_t \leq 1, \ for \ t=1,\cdots,T.
    \end{aligned}
\end{equation}

\begin{equation} \label{s2}
    \begin{aligned}
       max \ \ & (\frac{3}{4} - x_1)\mathbf{1}[x_1 \geq \frac{1}{2}] + \cdots + (\frac{3}{4} - x_{\frac{T}{2}})\mathbf{1}[x_{\frac{T}{2}} \geq \frac{1}{2}] \\
       & + (\frac{3}{4}-\frac{W_T}{T} - x_{\frac{T}{2}+1})\mathbf{1}[x_{\frac{T}{2}+1} \geq \frac{1}{2}] + \cdots + (\frac{3}{4}-\frac{W_T}{T} - x_T)\mathbf{1}[x_T \geq \frac{1}{2}] \\
       s.t. \ \ & \sum_{t=1}^T g_t(x_t)  \leq \frac{T}{4} , \ 0 \leq x_t \leq 1, \ for \ t=1,\cdots,T.
    \end{aligned}
\end{equation}

For any online policy, we denote $x_t^1(\pi)$ as the decision of policy $\pi$ at time period $t$ under the scenario given in (\ref{s1}) and $x_t^2(\pi)$ as the decision of policy $\pi$ at time period $t$ under the scenario given in (\ref{s2}). Then we define $T_1(\pi)$ and $T_2(\pi)$ as the number of $x_t$ which is no less than $\frac{1}{2}$ of policy $\pi$ under the two scenario during the first $T/2$ time periods:

\begin{equation*}
    T_1(\pi) = E [\sum_{t=1}^{\frac{T}{2}} \mathbf{1}[x_t^1 \geq \frac{1}{2}]] \ ,\ T_2(\pi) = E [\sum_{t=1}^{\frac{T}{2}} \mathbf{1}[x_t^2 \geq \frac{1}{2}]] .
\end{equation*}

Considering the budget constraint, we know that $T_1(\pi) \leq T/2$ and 
$T_2(\pi) \leq T/2$. Then we can calculate the expected reward collected by policy $\pi$ on both scenario:

\begin{equation*}
    \begin{aligned}
        & {ALG}_T^1(\pi) \leq T_1(\pi)(\frac{3}{4} - \frac{1}{2}) + (\frac{3}{4} - \frac{1}{2}+\frac{W_T}{T})(\frac{T}{2} - T_1(\pi)) = \frac{T}{8} + \frac{W_T}{2} - \frac{W_T}{T} \cdot T_1(\pi) \\
        & {ALG}_T^2(\pi) \leq T_2(\pi)(\frac{3}{4} - \frac{1}{2}) + (\frac{3}{4} - \frac{1}{2}-\frac{W_T}{T})(\frac{T}{2} - T_2(\pi)) = \frac{T}{8} - \frac{W_T}{2} + \frac{W_T}{T} \cdot T_2(\pi). 
    \end{aligned}
\end{equation*}

The offline optimal policy $\pi^\star$ who is aware of $v_t$ for each $t$ can achieve the objective value:

\begin{equation*}
    {ALG}_T^1(\pi^\star) = \frac{T}{8} + \frac{W_T}{2} \ , \ {ALG}_T^2(\pi^\star) = \frac{T}{8}.  
\end{equation*}

Thus the regret of policy $\pi$ on scenario (\ref{s1}) and (\ref{s2}) are no less than $\frac{W_T}{T} \cdot T_1(\pi)$ and $\frac{W_T}{2} - \frac{W_T}{T} \cdot T_2(\pi)$. Note that the implementation of policy $\pi$ at each time period should be independent of future realizations, we must have $T_1(\pi) = T_2(\pi)$. As a result, for any online policy $\pi$, we have

\begin{equation}
    {regret}(\pi;T) \geq max \left\{\frac{W_T}{T} \cdot T_1(\pi),  \frac{W_T}{2} - \frac{W_T}{T} \cdot T_1(\pi) \right\} \geq \frac{W_T}{4} = \Omega(W_T).
\end{equation}

\section{Proof of Lemma \ref{lem:decomposition}}
We first prove that $\mu^*$ is an optimal solution of $D_t(\mu)$ for all $t \in [T]$. To see this, note that for each $t$, $D_t(\mu)$ is a convex function of $\mu$ and
\[
\nabla D_t(\mu)=\rho_t+\nabla L(\mu,F_t)=\rho_t-\E_{v \sim F_t}\left[ x^*(v,\mu) G\big(x^*(v,\mu)\big) \right].
\]
With the definition of $\rho_t$ in \eqref{def:rho1}, it follows immediately that $\nabla D_t(\mu^*)=0$, which implies that $\mu^*$ is a minimizer of the function $D_t(\mu)$ for each $t$.

% We now prove that $\VLR(\mu^*)=\sum_{t=1}^{T}D_t(\mu^*)$.
%If $\mu^*=0$, then $\VLR(\mu^*)=\sum_{t=1}^{T}D_t(\mu^*)$ holds directly.\\
%If $\mu^*>0$, which implies that the budget constraint is binding. We have
%\[
%0=\nabla \VLR(\mu^*)=B-\E_{v \sim F}\left[ x^*(v,\mu)\big) G\big(x^*(v,\mu)\big) \right]=B-\sum_{t=1}^{T}\rho_t
%\]
%Thus, we have that
%\[
%B\cdot\mu^*=\sum_{t=1}^{T}\rho_t\cdot\mu^*
%\]
%It follows immediately that $\VLR(\mu^*)=\sum_{t=1}^{T}D_t(\mu^*)$.
Note that
\begin{equation*}
\begin{aligned}
\VLR(\mu^*) - \sum_{t=1}^{T}D_t(\mu^*) &= \left(B - \sum_{t=1}^{T}\rho_t\right) \mu^* \\
&= \left\{B - \sum_{t=1}^{T} \E_{v \sim F_t}\left[ x^*(v,\mu)\big) G\big(x^*(v,\mu)\big) \right] \right\} \mu^* \\
&= \nabla \VLR(\mu^*) \cdot \mu^* \\
&= 0
\end{aligned}
\end{equation*}
where the second equality follows from the definition of $\rho_t$ and the last equality follows from the optimality condition of $\mu^*$ that minimizes
the function $\VLR(\mu)$.

\section{Proof of \Cref{thrm:informative}}

The proof of \Cref{thrm:informative} is similar to the proof of \Cref{thrm:noninformative}, and the only difference is we substitute $\rho$ for $\hat{\rho}_t$ in this section. We consider the upper bound on term $(a)$ and $(b)$ respectively.

\subsection{Upper Bound on Term $(a)$}\label{appx:subsec:term-a-informative}

Similar to \eqref{eq:tmp7}, we have
\begin{equation}\label{eq:tmp7Info}
\begin{aligned}
(a) \leq& \VOPT - \E\left[\sum_{t=1}^T f^*(v_t, \muR_t) + \muR_t \hat{\rho}_t \right]
+ \E\left[\sum_{t=1}^T \muR_t (\hat{\rho}_t - \xR_t G(\xR_t))\right] + 2b \cdot \E\left[\sum_{t=1}^{T} err_G(t)\right] \\
\leq& \underbrace{\VOPT - \E\left[\sum_{t=1}^T f^*(v_t, \muR_t) + \muR_t \hat{\rho}_t \right]}_{(c)}
+ \underbrace{\E\left[\sum_{t=1}^T \muR (\hat{\rho}_t - \xR_t \mathbf{1}[\xR_t \geq m_t])\right]}_{(d)} + O(\sqrt{T \ln T})
\end{aligned}
\end{equation}

\paragraph{Upper Bound on Term $(c)$.}
Since $\muR_t$ and $v_t$ are independent, we have $\E[f^*(v_t, \muR_t)] = \E_{\muR_t}\big[ L(\muR_t, F_t) \big]$ with function $L(\mu,F)$ defined in (\ref{eq:def-L}). Thus,
\begin{equation}\label{eq:tmp3Info}
\E\left[\sum_{t=1}^T \big(f^*(v_t, \muR_t) + \muR_t \hat{\rho}_t\big) \right] =
\E\left[\sum_{t=1}^T \big(L(\muR_t, F_t) + \muR_t \hat{\rho}_t \big) \right].
\end{equation}
On the other hand, note that $\VOPT \leq \VLR(\mu)$ for any $\mu \geq 0$ (Lemma \ref{lemma:weak-duality}). From Lemma \ref{lem:decomposition}, we know
\begin{equation}\label{eq:tmp4Info}
V^{\text{OPT}}\leq \min_{\mu\geq0}V^{\text{LR}}(\mu)=\sum_{t\in[T]}\min_{\mu_t\geq0}D_t(\mu_t)\leq \sum_{t\in[T]} \E_{\muR_t}\big[ D_t(\muR_t)\big]=\E\left[\sum_{t=1}^T \Big(L(\muR_t, F_t) + \muR_t \rho_t \Big) \right]
\end{equation}
with $\rho_t$ defined in \eqref{def:rho1}.
From (\ref{eq:tmp3Info}) and (\ref{eq:tmp4Info}), we have
\begin{equation}\label{eq:tmp5Info}
(c) \leq \sum_{t=1}^{T} \E\big[\muR_t\rho_t-\muR_t\hat{\rho}_t\big]\leq(b/a+b)\cdot\sum_{t=1}^{T}\E|\rho_t-\hat{\rho}_t| = O\big(V_T\big)
\end{equation}
where the last equality follows from the definition of $V_T$ in \eqref{eqn:DeviationRho}.

\paragraph{Upper Bound on Term $(d)$.}
Similar to proof of \Cref{thrm:noninformative}, we have
\begin{equation*}
\begin{aligned}
\sum_{t=1}^T \muR (\hat{\rho}_t - \xR_t \mathbf{1}[\xR_t \geq m_t]) \leq \frac{b^2}{2} \cdot \eta T + \frac{\mu_1^2}{2\eta}.
\end{aligned}
\end{equation*}
Therefore, by taking $\eta = \frac{1}{\sqrt{T}}$,
\begin{equation}\label{eq:tmp6Info}
(d) \leq \frac{b^2}{2} \cdot \eta T + \frac{\mu_1^2}{2\eta} = O(\sqrt{T}).
\end{equation}
From (\ref{eq:tmp7Info}), (\ref{eq:tmp5Info}), and (\ref{eq:tmp6Info}), we have
\begin{equation*}
(a) = O(\sqrt{T} + V_T).
\end{equation*}

\subsection{Upper Bound on Term $(b)$}\label{appx:subsec:term-b-informative}
Note that $\muR_{t+1} = (\muR_t - \eta g_t)^{+} \geq \muR_t - \eta g_t = \muR_t - \eta (\hat{\rho}_t - \zR_t)$
and $\nabla \VLR(\mu^*) = B - \sum_{t=1}^{T}{\rho}_t \geq 0$ by the optimality condition of $\mu^*$. Therefore, we have
\begin{equation*}
\begin{aligned}
\sum_{t=1}^T \zR_t - B 
&\leq \sum_{t=1}^T \big(\zR_t - \hat{\rho}_t \big) + \sum_{t=1}^T |\hat{\rho}_t - {\rho}_t| \\
&\leq \frac{\muR_{T+1} - \mu_1}{\eta} +  V_T.
\end{aligned}
\end{equation*}
As a result, with $\muR_t \leq \frac{b}{a}+b$ for all $t$ by Lemma \ref{lemma:bdd-mu}, by taking step size $\eta = \frac{1}{\sqrt{T}}$ , we have
\begin{equation*}
(b) = O(\sqrt{T}+V_T).
\end{equation*}

\section{Proof of Proposition \ref{prop:lbd-V}}
The proof of Proposition \ref{prop:lbd-V} is similar to that of Proposition \ref{prop:lbd-W}.To simplify the proof, here we assume $a=0, b=1$, and denote the reward and consumption at each time period $t$ as $f_t(x_t) = (v_t - x_t) \cdot \mathbf{1}[x_t \geq m_t]$ and $g_t(x_t) = x_t \mathbf{1}[x_t \geq m_t] = z_t$.

Set the budget constraint $B = T/4$. We assume $m_t = \frac{1}{2}$ for each $t$ and offer the prediction of $\rho_t$ as $\hat{\rho}_t = \frac{1}{2}$ when $t$ is odd and $\hat{\rho}_t = 0$ when $t$ is even. Without loss of generality, we assume $V_T$ is an integer and $V_T \leq T/2$. Now we consider the following two scenario. The first one, given in (\ref{s1}), is that $v_t = \frac{3}{4}$ for $t=1, \cdots, T-V_T$ and $v_t = \frac{7}{8} $ for $t=T+1-V_T, \cdots, T$. The second scenario, given in (\ref{s2}), is that $v_t = \frac{3}{4}$ for $t=1, \cdots, T-V_T$ and $v_t = \frac{5}{8} $ for $t=T+1-V_T, \cdots, T$.

\begin{equation} \label{senario1}
    \begin{aligned}
       max \ \ & (\frac{3}{4} - x_1)\mathbf{1}[x_1 \geq \frac{1}{2}] + \cdots + (\frac{3}{4} - x_{T-V_T})\mathbf{1}[x_{T-V_T} \geq \frac{1}{2}] \\
       + & (\frac{7}{8} - x_{T+1-V_T})\mathbf{1}[x_{T+1-V_T} \geq \frac{1}{2}] + \cdots + (\frac{7}{8} - x_T)\mathbf{1}[x_T \geq \frac{1}{2}] \\
       s.t. \ \ & \sum_{t=1}^T z_t \leq \frac{T}{4}, \ 0 \leq x_t \leq 1, \ for \ t=1,\cdots,T.
    \end{aligned}
\end{equation}

\begin{equation} \label{senario2}
    \begin{aligned}
       max \ \ & (\frac{3}{4} - x_1)\mathbf{1}[x_1 \geq \frac{1}{2}] + \cdots + (\frac{3}{4} - x_{T-V_T})\mathbf{1}[x_{T-V_T} \geq \frac{1}{2}] \\
       + & (\frac{5}{8} - x_{T+1-V_T})\mathbf{1}[x_{T+1-V_T} \geq \frac{1}{2}] + \cdots + (\frac{5}{8} - x_T)\mathbf{1}[x_T \geq \frac{1}{2}] \\
       s.t. \ \ & \sum_{t=1}^T z_t \leq \frac{T}{4}, \ 0 \leq x_t \leq 1, \ for \ t=1,\cdots,T.
    \end{aligned}
\end{equation}
where $z_t = x_t \mathbf{1}[x_t \geq \frac{1}{2}]$ for each $t$. In scenario one, we can obtain that $\rho_t^1 = \frac{1}{2}$ when $t \geq T+1-V_T$, while in scenario two, $\rho_t^2 = 0$ when $t \geq T+1-V_T$. For $t \leq T-V_T$, we arrange the rest of budget to minimize $ V_T^1 = \sum_{t=1}^T |\rho_t^1 - \hat{\rho_t}|$ and $V_T^2 = \sum_{t=1}^T |\rho_t^2 - \hat{\rho_t}|$ and we have $V_T^1 = V_T^2 = V_T/2$.

For any online policy, we denote $x_t^1(\pi)$ as the decision of policy $\pi$ at time period $t$ under the scenario given in (\ref{senario1}) and $x_t^2(\pi)$ as the decision of policy $\pi$ at time period $t$ under the scenario given in (\ref{senario2}). Then we define $T_1(\pi)$ and $T_2(\pi)$ as the number of $x_t$ which is no less than $\frac{1}{2}$ of policy $\pi$ under the two scenario during the first $T-V_T$ time periods:

\begin{equation*}
    T_1(\pi) = E [\sum_{t=1}^{T-V_T} \mathbf{1}[x_t^1 \geq \frac{1}{2}]] \ ,\ T_2(\pi) = E [\sum_{t=1}^{T-V_T} \mathbf{1}[x_t^2 \geq \frac{1}{2}]] 
\end{equation*}

With budget constraint, we know that $T/2-V_T \leq T_1(\pi) \leq T/2$ and 
$T_2(\pi) \leq T/2$. We can calculate the expected reward collected by policy $\pi$ on both scenario:

\begin{equation*}
    \begin{aligned}
        & {ALG}_T^1(\pi) \leq T_1(\pi)(\frac{3}{4} - \frac{1}{2}) + (\frac{T}{2} - T_1(\pi))(\frac{7}{8} - \frac{1}{2}) = \frac{3T}{16} - \frac{1}{8} \cdot T_1(\pi) \\
        & {ALG}_T^2(\pi) \leq T_2(\pi)(\frac{3}{4} - \frac{1}{2}) + (\frac{T}{2} - T_2(\pi))(\frac{5}{8} - \frac{1}{2})  = \frac{T}{16} + \frac{1}{8} \cdot T_2(\pi)
    \end{aligned}
\end{equation*}
Note that the offline optimal policy $\pi^\star$ who is aware of $v_t$ for each $t$ can achieve the objective value:

\begin{equation*}
    {ALG}_T^1(\pi^\star) = \frac{T}{8} + \frac{V_T}{8} \ , \ {ALG}_T^2(\pi^\star) = \frac{T}{8} 
\end{equation*}

Thus we have the lower bound for regret of policy $\pi$ on scenario (\ref{s1}) and (\ref{s2}) respectively:
\begin{equation*}
    {regret}_T^1(\pi) \geq \frac{V_T}{8} - \frac{T}{16} + \frac{T_1(\pi)}{8} \ , \ {regret}_T^2(\pi) \geq \frac{T}{16} - \frac{T_2(\pi)}{8} 
\end{equation*}
 Note that the implementation of policy $\pi$ at each time period should be independent of future realizations, we must have $T_1(\pi) = T_2(\pi)$. As a result, for any online policy $\pi$, we have the conclusion:

\begin{equation}
    {regret}(\pi;T) \geq max \left\{ \frac{V_T}{8} - \frac{T}{16} + \frac{T_1(\pi)}{8},  \frac{T}{16} - \frac{T_2(\pi)}{8}\right\} \geq \frac{V_T}{16} \geq \Omega(V_T) 
\end{equation}
